# Supplementary material for: Coupled-cluster theory for atoms and molecules in strong magnetic fields
Source: arXiv:1505.08045 source file (2015-08-12)
Supplement: Supplementary file 1 [file SI.pdf]

**Coupled-cluster theory for atoms and molecules in strong magnetic fields**

**SUPPLEMENTARY MATERIAL**

Stella Stopkowicz,[1, a)] Jürgen Gauss,[2] Kai K. Lange,[1] Erik I. Tellgren,[1] and Trygve Helgaker[1]

[1)] *Centre for Theoretical and Computational Chemistry (CTCC), Department of Chemistry, University of Oslo, P.O.Box 1033 Blindern, 0315 Oslo, Norway*

[2)] *Institut für Physikalische Chemie, Universität Mainz, D-55099 Mainz, Germany*

[a)] Electronic mail: stella.stopkowicz@kjemi.uio.no

TABLE I. HF-SCF and FCI energies (in Hartree) for helium as a function of the magnetic field for the $^1$S and $^3$P states calculated with the uncontracted d-aug-cc-pVQZ basis set.

| | $^1$S state | | $^3$P state | |
|---|---|---|---|---|
| B/$B_0$ | HF-SCF | FCI | HF-SCF | FCI |
| 0.0 | -2.861547 | -2.902836 | -2.128973 | -2.130862 |
| 0.1 | -2.859576 | -2.900849 | -2.258697 | -2.260884 |
| 0.2 | -2.853711 | -2.894940 | -2.359530 | -2.362424 |
| 0.3 | -2.844082 | -2.885245 | -2.449269 | -2.452840 |
| 0.4 | -2.830875 | -2.871958 | -2.533595 | -2.537685 |
| 0.5 | -2.814306 | -2.855304 | -2.613142 | -2.617648 |
| 0.6 | -2.794602 | -2.835514 | -2.688493 | -2.693342 |
| 0.8 | -2.746663 | -2.787419 | -2.828330 | -2.833704 |
| 1.0 | -2.688682 | -2.729313 | -2.955373 | -2.961129 |
| 1.2 | -2.622020 | -2.662561 | -3.072129 | -3.078170 |

TABLE II. HF-SCF, CCSD, and CCSD(T) energies (in Hartree) for neon as a function of the magnetic field for the $^1$S, $^3$P, $^3$D, and $^3$F states calculated with the uncontracted aug-cc-pCVQZ basis set.

| | | $^1$S state | | | $^3$P state | |
|---|---|---|---|---|---|---|
| B/$B_0$ | HF-SCF | CCSD | CCSD(T) | HF-SCF | CCSD | CCSD(T) |
| 0.0 | -128.546441 | -128.914514 | -128.921003 | -127.969192 | -128.283553 | -128.287974 |
| 0.1 | -128.538641 | -128.906570 | -128.913033 | -128.102421 | -128.416961 | -128.421389 |
| 0.2 | -128.515343 | -128.882859 | -128.889250 | -128.203383 | -128.518457 | -128.522907 |
| 0.3 | -128.476841 | -128.843712 | -128.849994 | -128.275784 | -128.591702 | -128.596185 |
| 0.4 | -128.423558 | -128.789604 | -128.795751 | -128.325183 | -128.642119 | -128.646636 |
| 0.5 | -128.356002 | -128.721091 | -128.727086 | -128.357745 | -128.675634 | -128.680169 |
| 0.6 | -128.274724 | -128.638768 | -128.644602 | -128.378687 | -128.697216 | -128.701739 |
| 0.8 | -128.073286 | -128.435104 | -128.440614 | -128.396826 | -128.715400 | -128.719801 |
| 1.0 | -127.823749 | -128.183333 | -128.188533 | -128.385756 | -128.703415 | -128.707633 |
| 1.2 | -127.530328 | -127.887796 | -127.892715 | | | |
| | | $^3$D state | | | $^3$F state | |
| B/$B_0$ | HF-SCF | CCSD | CCSD(T) | HF-SCF | CCSD | CCSD(T) |
| 0.0 | -127.888220 | -128.197613 | -128.201628 | | | |
| 0.1 | -128.065017 | -128.374562 | -128.378581 | | | |
| 0.2 | -128.197112 | -128.507159 | -128.511195 | | | |
| 0.3 | -128.289857 | -128.600868 | -128.604937 | -128.073856 | -128.390027 | -128.394324 |
| 0.4 | -128.352224 | -128.664705 | -128.668826 | -128.229327 | -128.545566 | -128.549831 |
| 0.5 | -128.394534 | -128.708777 | -128.712957 | -128.359617 | -128.675999 | -128.680228 |
| 0.6 | -128.423897 | -128.739812 | -128.744038 | -128.466139 | -128.782769 | -128.786962 |
| 0.8 | -128.449218 | -128.767664 | -128.771920 | -128.615268 | -128.932796 | -128.936923 |
| 0.9 | -128.443890 | -128.763342 | -128.767595 | | | |
| 1.0 | | | | -128.694447 | -129.013409 | -129.017484 |
| 1.2 | | | | -128.723219 | -129.043843 | -129.047870 |

TABLE III. HF-SCF, CCSD, and CCSD(T) energies (in Hartree) for fluorine as a function of the magnetic field for the $^2$P, $^2$G, $^4$P, $^4$D, and $^4$F states calculated with the uncontracted aug-cc-pCVQZ basis set.

| | | $^2$P state | | | | |
|---|---|---|---|---|---|---|
| B/$B_0$ | HF-SCF | CCSD | CCSD(T) | | | |
| 0.00002 | -99.411605 | -99.715113 | -99.720724 | | | |
| 0.0002 | -99.411785 | -99.715293 | -99.720904 | | | |
| 0.002 | -99.413581 | -99.717090 | -99.722701 | | | |
| 0.02 | -99.431255 | -99.734757 | -99.740367 | | | |
| 0.04 | -99.450264 | -99.753749 | -99.759355 | | | |
| 0.06 | -99.468614 | -99.772070 | -99.777670 | | | |
| 0.08 | -99.486306 | -99.789721 | -99.795313 | | | |
| 0.1 | -99.503341 | -99.806704 | -99.812287 | | | |
| 0.2 | -99.578767 | -99.881717 | -99.887222 | | | |
| 0.3 | -99.638291 | -99.940613 | -99.946004 | | | |
| 0.4 | -99.682514 | -99.984059 | -99.989312 | | | |
| 0.5 | -99.712130 | -100.012804 | -100.017909 | | | |
| 0.6 | -99.727871 | -100.027625 | -100.032579 | | | |
| 0.8 | -99.720630 | -100.018533 | -100.023192 | | | |
| 1.0 | -99.666297 | -99.962467 | -99.966858 | | | |
| 1.2 | -99.569737 | -99.864365 | -99.868521 | | | |
| 1.4 | -99.435126 | -99.728421 | -99.732373 | | | |
| 1.6 | -99.266029 | -99.558189 | -99.561961 | | | |
| | | $^2$G state | | | $^4$P state | |
| B/$B_0$ | HF-SCF | CCSD | CCSD(T) | HF-SCF | CCSD | CCSD(T) |
| 0 | | | | -98.987865 | -99.239364 | -99.243092 |
| 0.00002 | | | | -98.987905 | -99.239404 | -99.243132 |
| 0.0002 | | | | -98.988265 | -99.239764 | -99.243492 |
| 0.002 | | | | -98.991857 | -99.243356 | -99.247084 |
| 0.02 | | | | -99.027062 | -99.278574 | -99.282303 |
| 0.04 | | | | -99.064657 | -99.316209 | -99.319940 |
| 0.06 | | | | -99.100665 | -99.352283 | -99.356018 |
| 0.08 | | | | -99.135107 | -99.386818 | -99.390559 |
| 0.1 | | | | -99.168017 | -99.419847 | -99.423594 |
| 0.2 | | | | -99.311262 | -99.564041 | -99.567844 |
| 0.3 | | | | -99.425123 | -99.679256 | -99.683134 |
| 0.4 | | | | -99.518972 | -99.774428 | -99.778367 |
| 0.5 | -99.347103 | -99.612660 | -99.616326 | -99.600163 | -99.856514 | -99.860474 |
| 0.6 | -99.434914 | -99.701306 | -99.704967 | -99.672163 | -99.928906 | -99.932842 |
| 0.8 | -99.553643 | -99.822248 | -99.825910 | -99.788896 | -100.045679 | -100.049509 |
| 1 | -99.621752 | -99.892633 | -99.896284 | -99.863826 | -100.120711 | -100.124444 |
| 1.2 | -99.657272 | -99.929798 | -99.933398 | | | |
| 1.4 | -99.664560 | -99.938082 | -99.941600 | | | |
| 1.6 | -99.643949 | -99.918070 | -99.921491 | | | |
| | | $^4$D state | | | $^4$F state | |
| B/$B_0$ | HF-SCF | CCSD | CCSD(T) | HF-SCF | CCSD | CCSD(T) |
| 0.1 | | | | -99.137253 | -99.384241 | -99.387555 |
| 0.2 | -99.122456 | -99.375329 | -99.378921 | -99.306905 | -99.554789 | -99.558142 |
| 0.3 | -99.338746 | -99.591914 | -99.595491 | -99.435545 | -99.685054 | -99.688475 |
| 0.4 | -99.523929 | -99.777575 | -99.781140 | -99.538411 | -99.789983 | -99.793489 |
| 0.5 | -99.680481 | -99.934836 | -99.938392 | -99.625546 | -99.879065 | -99.882641 |
| 0.6 | -99.811662 | -100.066984 | -100.070538 | -99.699020 | -99.954198 | -99.957822 |
| 0.8 | -100.013899 | -100.271820 | -100.275390 | -99.804357 | -100.062450 | -100.066142 |
| 0.9 | | | | -99.838152 | -100.097640 | -100.101364 |
| 0.95 | | | | -99.851063 | -100.111233 | -100.114974 |
| 1.0 | -100.161892 | -100.422620 | -100.426204 | | | |
| 1.2 | -100.274554 | -100.537546 | -100.541114 | | | |
| 1.4 | -100.356684 | -100.621357 | -100.624884 | | | |
| 1.6 | -100.408771 | -100.674800 | -100.678275 | | | |

TABLE IV. HF-SCF and CCSD(T) energies (in Hartree) for lithium as a function of the magnetic field for the $^2$S and $^2$P calculated with the uncontracted aug-cc-pCVQZ basis set.

| | $^2$S state | | $^2$P state | |
|---|---|---|---|---|
| B/$B_0$ | HF-SCF | CCSD(T) | HF-SCF | CCSD(T) |
| 0.00 | -7.432725 | -7.476841 | | |
| 0.02 | -7.442107 | -7.486232 | -7.383923 | -7.427797 |
| 0.04 | -7.450286 | -7.494434 | -7.400688 | -7.444638 |
| 0.06 | -7.457344 | -7.501529 | -7.415681 | -7.459738 |
| 0.08 | -7.463389 | -7.507621 | -7.429245 | -7.473431 |
| 0.10 | -7.468533 | -7.512818 | -7.441659 | -7.485985 |
| 0.20 | -7.483917 | -7.528508 | -7.492110 | -7.537222 |
| 0.30 | -7.487686 | -7.532573 | -7.530447 | -7.576381 |
| 0.40 | -7.484406 | -7.529538 | -7.561424 | -7.608157 |
| 0.50 | -7.476543 | -7.521859 | -7.587181 | -7.634663 |
| 0.60 | -7.465385 | -7.510833 | -7.608737 | -7.656915 |
| 0.80 | -7.435372 | -7.480998 | -7.641654 | -7.691062 |
| 1.00 | -7.396960 | -7.442729 | -7.663560 | -7.713979 |
| 1.20 | -7.352019 | -7.397916 | -7.675791 | -7.727029 |
| 1.40 | -7.301657 | -7.347658 | -7.678587 | -7.730503 |
| 1.60 | -7.245767 | -7.291846 | -7.672125 | -7.724624 |

TABLE V. HF-SCF, CCSD, and CCSD(T) energies (in Hartree) for beryllium as a function of the magnetic field for the $^1$S, $^1$D, and $^3$P states calculated with the uncontracted aug-cc-pCVQZ basis set.

| | | $^1$S state | | | $^1$D state | |
|---|---|---|---|---|---|---|
| B/$B_0$ | HF-SCF | CCSD | CCSD(T) | HF-SCF | CCSD | CCSD(T) |
| 0.0 | -14.572986 | -14.665197 | -14.665797 | -14.302915 | -14.402637 | -14.404060 |
| 0.00005 | | | | -14.302965 | -14.402687 | -14.404110 |
| 0.005 | -14.572952 | -14.665164 | -14.665764 | | | |
| 0.05 | | | | -14.347049 | -14.446334 | -14.447660 |
| 0.01 | -14.572848 | -14.665067 | -14.665667 | | | |
| 0.02 | -14.572410 | -14.664655 | -14.665255 | | | |
| 0.04 | -14.570688 | -14.663036 | -14.663638 | | | |
| 0.06 | -14.567843 | -14.660358 | -14.660963 | | | |
| 0.08 | -14.563910 | -14.656650 | -14.657260 | | | |
| 0.1 | -14.558931 | -14.651951 | -14.652565 | -14.380443 | -14.478651 | -14.479766 |
| 0.12 | -14.552955 | -14.646300 | -14.646921 | | | |
| 0.14 | -14.546033 | -14.639744 | -14.640372 | | | |
| 0.16 | -14.538213 | -14.632329 | -14.632965 | | | |
| 0.18 | -14.529546 | -14.624099 | -14.624744 | | | |
| 0.2 | -14.520079 | -14.615099 | -14.615754 | -14.422900 | -14.519151 | -14.519933 |
| 0.3 | -14.462202 | -14.559979 | -14.560698 | -14.442910 | -14.538437 | -14.539091 |
| 0.4 | -14.389953 | -14.491200 | -14.492014 | -14.447377 | -14.542751 | -14.543353 |
| 0.5 | -14.306706 | -14.412280 | -14.413234 | | | |
| 0.6 | -14.214904 | -14.325897 | -14.327057 | -14.424397 | -14.519923 | -14.520483 |
| 0.7 | -14.116339 | -14.234125 | -14.235587 | | | |
| 0.8 | | | | -14.372883 | -14.468579 | -14.469121 |
| 1.0 | | | | -14.301402 | -14.397184 | -14.397715 |
| 1.2 | | | | -14.214090 | -14.309936 | -14.310458 |
| 1.4 | | | | -14.113682 | -14.209575 | -14.210088 |
| 1.6 | | | | -14.002329 | -14.098221 | -14.098726 |

| | | $^3$P state | |
|---|---|---|---|
| B/$B_0$ | HF-SCF | CCSD | CCSD(T) |
| 0.0 | -14.513675 | -14.565596 | -14.565680 |
| 0.05 | -14.582748 | -14.636354 | -14.636449 |
| 0.1 | -14.645411 | -14.699109 | -14.699204 |
| 0.2 | -14.750560 | -14.804606 | -14.804703 |
| 0.3 | -14.835106 | -14.889660 | -14.889760 |
| 0.4 | -14.904457 | -14.959619 | -14.959725 |
| 0.5 | -14.962258 | -15.018093 | -15.018205 |
| 0.6 | -15.011087 | -15.067637 | -15.067756 |
| 0.8 | -15.088755 | -15.146804 | -15.146937 |
| 1.0 | -15.147047 | -15.206612 | -15.206760 |
| 1.2 | -15.191255 | -15.252290 | -15.252453 |
| 1.4 | -15.224601 | -15.287024 | -15.287199 |
| 1.6 | -15.249259 | -15.312963 | -15.313151 |

TABLE VI. HF-SCF, CCSD, and CCSD(T) energies (in Hartree) for sodium as a function of the magnetic field for the $^2$S, $^2$P, $^2$D, and $^2$F states calculated with the uncontracted aug-cc-pCVQZ basis set.

| | | $^2$S state | | | $^2$P state | |
|---|---|---|---|---|---|---|
| B/$B_0$ | HF-SCF | CCSDR | CCSD(T) | HF-SCF | CCSD | CCSD(T) |
| 0 | -161.858733 | -162.221743 | -162.226265 | -161.786251 | -162.145306 | -162.149565 |
| 0.000000001 | | | | -161.786251 | -162.145306 | -162.149565 |
| 0.005 | -161.861178 | -162.224191 | -162.228713 | | | |
| 0.01 | -161.863516 | -162.226534 | -162.231056 | | | |
| 0.02 | -161.867832 | -162.230873 | -162.235397 | | | |
| 0.04 | -161.875175 | -162.238302 | -162.242831 | | | |
| 0.06 | -161.880876 | -162.244132 | -162.248667 | | | |
| 0.08 | -161.885076 | -162.248490 | -162.253034 | | | |
| 0.1 | -161.887916 | -162.251505 | -162.256058 | -161.848609 | -162.208473 | -162.212774 |
| 0.12 | -161.889524 | -162.253296 | -162.257858 | | | |
| 0.14 | -161.890009 | -162.253965 | -162.258536 | | | |
| 0.16 | -161.889465 | -162.253602 | -162.258182 | | | |
| 0.18 | -161.887972 | -162.252285 | -162.256872 | | | |
| 0.2 | -161.885600 | -162.250079 | -162.254672 | -161.867394 | -162.228403 | -162.232755 |
| 0.3 | -161.862414 | -162.227525 | -162.232136 | -161.860966 | -162.223080 | -162.227471 |
| 0.4 | -161.823719 | -162.189084 | -162.193684 | -161.835545 | -162.198643 | -162.203057 |
| 0.5 | -161.772258 | -162.137541 | -162.142105 | -161.793826 | -162.157772 | -162.162196 |
| 0.6 | -161.709368 | -162.074349 | -162.078860 | -161.737236 | -162.101925 | -162.106348 |
| 0.7 | -161.635781 | -162.000344 | -162.004794 | -161.667072 | -162.032402 | -162.036814 |
| 0.8 | -161.552007 | -161.916096 | -161.920480 | -161.584441 | -161.950293 | -161.954685 |
| 0.9 | -161.458504 | -161.822083 | -161.826398 | -161.490006 | -161.856256 | -161.860620 |
| 1.0 | -161.355560 | -161.718601 | -161.722845 | -161.383966 | -161.750504 | -161.754833 |
| 1.1 | -161.243314 | -161.605794 | -161.609967 | -161.266235 | -161.632983 | -161.637272 |
| 1.2 | -161.121783 | -161.483686 | -161.487787 | | | |
| 1.3 | -160.990916 | -161.352238 | -161.356267 | | | |
| 1.4 | -160.850660 | -161.211402 | -161.215361 | | | |
| | | $^2$D state | | | $^2$F state | |
| B/$B_0$ | HF-SCF | CCSD | CCSD(T) | HF-SCF | CCSD | CCSD(T) |
| 0.05 | -161.782186 | -162.139903 | -162.144087 | | | |
| 0.1 | -161.808840 | -162.166986 | -162.171197 | -161.769617 | -162.127152 | -162.131322 |
| 0.2 | -161.837229 | -162.196436 | -162.200709 | -161.797305 | -162.155067 | -162.159249 |
| 0.3 | -161.846522 | -162.206837 | -162.211162 | -161.792585 | -162.150834 | -162.155041 |
| 0.4 | -161.840093 | -162.201510 | -162.205876 | -161.777062 | -162.135724 | -162.139947 |
| 0.5 | -161.820098 | -162.182561 | -162.186952 | -161.743514 | -162.102648 | -162.106885 |
| 0.6 | -161.788631 | -162.151975 | -162.156372 | -161.698577 | -162.058087 | -162.062328 |
| 0.7 | -161.746363 | -162.110375 | -162.114757 | -161.643109 | -162.002684 | -162.006904 |
| 0.8 | -161.692976 | -162.057468 | -162.061819 | -161.571168 | -161.930520 | -161.934700 |
| 0.9 | | | | -161.476995 | -161.835947 | -161.840075 |
| 1.0 | -161.550819 | -161.915901 | -161.920159 | -161.357045 | -161.715503 | -161.719575 |
| 1.1 | | | | -161.209410 | -161.567333 | -161.571349 |
| 1.2 | -161.360020 | -161.725512 | -161.729658 | | | |
| 1.4 | -161.122593 | -161.488610 | -161.492643 | | | |
| 1.6 | -160.844830 | -161.211646 | -161.215573 | | | |

TABLE VII. Potential-energy curves for the lowest singlet and triplet states of LiH without magnetic field with R as the bond distance (in Bohr). Calculated at the CCSD(T) level with the uncontracted aug-cc-pVTZ basis set.

| | | | B=0 $B_0$ | | |
|---|---|---|---|---|---|
| R | $^3\Pi$ | R | $^1\Sigma$ | R | $^3\Sigma$ |
| 1.4 | -7.624431 | 1.4 | -7.762607 | 1.4 | -7.661501 |
| 1.6 | -7.717706 | 1.6 | -7.869961 | 1.6 | -7.752312 |
| 1.8 | -7.781722 | 1.8 | -7.942485 | 1.8 | -7.814812 |
| 2 | -7.825766 | 2.0 | -7.990829 | 2.0 | -7.858119 |
| 2.2 | -7.855986 | 2.2 | -8.022338 | 2.2 | -7.888245 |
| 2.4 | -7.876563 | 2.4 | -8.042112 | 2.4 | -7.909264 |
| 2.6 | -7.890381 | 2.6 | -8.053693 | 2.6 | -7.923969 |
| 2.8 | -7.899452 | 2.8 | -8.059553 | 2.8 | -7.934297 |
| 3 | -7.905198 | 3.0 | -8.061431 | 3.0 | -7.941600 |
| 3.2 | -7.908630 | 3.0191 | -8.061450 | 3.0191 | -7.942176 |
| 3.4 | -7.910470 | 3.0248 | -8.061451 | 3.0248 | -7.942346 |
| 3.6 | -7.911237 | 3.2 | -8.060556 | 3.2 | -7.946827 |
| 3.65 | -7.911306 | 3.4 | -8.057803 | 3.4 | -7.950640 |
| 3.7 | -7.911337 | 3.6 | -8.053793 | 3.6 | -7.953500 |
| 3.7185 | -7.911339 | 3.8 | -8.048974 | 3.8 | -7.955720 |
| 3.75 | -7.911332 | 4.0 | -8.043668 | 4.0 | -7.957515 |
| 3.8 | -7.911297 | 4.2 | -8.038108 | 4.2 | -7.959025 |
| 3.85 | -7.911235 | 4.6 | -8.026851 | 4.6 | -7.961509 |
| 3.9 | -7.911149 | 4.8 | -8.021368 | 4.8 | -7.962567 |
| 3.95 | -7.911042 | 5.0 | -8.016076 | 5.0 | -7.963531 |
| 4 | -7.910916 | 5.2 | -8.011026 | 5.2 | -7.964407 |
| 4.2 | -7.910278 | 5.4 | -8.006252 | 5.4 | -7.965201 |
| 4.6 | -7.908701 | | | | |
| 4.8 | -7.907903 | | | | |
| 5 | -7.907151 | | | | |
| 5.2 | -7.906465 | | | | |
| 5.4 | -7.905850 | | | | |

TABLE VIII. Potential-energy curves for the lowest singlet and triplet states of LiH in a magnetic field of 0.1 $B_0$ with R as the bond distance (in Bohr). Calculated at the CCSD(T) level with the uncontracted aug-cc-pVTZ basis set in a field perpendicular and parallel to the molecular bond axis.

| | | | B=0.1 $B_0$ | | | | |
|---|---|---|---|---|---|---|---|
| R | singlet$^{\perp}$ | R | $^1\Sigma^{\parallel}$ | R | triplet$^{\perp}$ | R | $^3\Pi^{\parallel}$ |
| 1.4 | -7.762001 | 1.4 | -7.753641 | 1.4 | -7.760805 | 1.4 | -7.755434 |
| 1.6 | -7.868205 | 1.6 | -7.861300 | 1.6 | -7.851338 | 1.6 | -7.848053 |
| 1.8 | -7.939779 | 1.8 | -7.933899 | 1.8 | -7.913669 | 1.8 | -7.911464 |
| 2.0 | -7.987300 | 2.0 | -7.982185 | 2.0 | -7.956776 | 2.0 | -7.954943 |
| 2.2 | -8.018067 | 2.2 | -8.013559 | 2.2 | -7.986607 | 2.2 | -7.984627 |
| 2.4 | -8.037005 | 2.4 | -8.033148 | 2.4 | -8.007213 | 2.4 | -8.004695 |
| 2.6 | -8.048075 | 2.6 | -8.044515 | 2.6 | -8.021385 | 2.6 | -8.018032 |
| 2.8 | -8.053303 | 2.8 | -8.050142 | 2.8 | -8.031071 | 2.8 | -8.026652 |
| 2.9801 | -8.054579 | 3.0191 | -8.051771 | 3.0 | -8.038144 | 3.0 | -8.031978 |
| 3.0 | -8.054565 | 3.0248 | -8.051765 | 3.0191 | -8.038292 | 3.0191 | -8.032354 |
| 3.0191 | -8.054526 | 3.0 | -8.051775 | 3.0248 | -8.037642 | 3.0248 | -8.032463 |
| 3.0248 | -8.054510 | 3.0035 | -8.051776 | 3.2 | -8.042068 | 3.2 | -8.035025 |
| 3.2 | -8.053086 | 3.2 | -8.050649 | 3.4 | -8.045035 | 3.4 | -8.036517 |
| 3.4 | -8.049737 | 3.4 | -8.047639 | 3.6 | -8.047023 | 3.6 | -8.036971 |
| 3.6 | -8.045139 | 3.6 | -8.043370 | 3.8 | -8.048371 | 3.6237 | -8.036975 |
| 3.8 | -8.039736 | 3.8 | -8.038289 | 4.0 | -8.049309 | 3.8 | -8.036759 |
| 4.0 | -8.033847 | 4.0 | -8.032720 | 4.2 | -8.049995 | 4.0 | -8.036142 |
| 4.2 | -8.027700 | 4.2 | -8.026893 | 4.6 | -8.050976 | 4.2 | -8.035304 |
| 4.6 | -8.015247 | 4.6 | -8.015093 | 4.8 | -8.051370 | 4.4 | -8.034372 |
| 4.8 | -8.009148 | 4.8 | -8.009332 | 5.0 | -8.051731 | 4.6 | -8.033427 |
| 5.0 | -8.003225 | 5.0 | -8.003758 | 5.2 | -8.052063 | 4.8 | -8.032522 |
| 5.2 | -7.997525 | 5.2 | -7.998418 | 5.4 | -8.052369 | 5.0 | -8.031687 |
| 5.4 | -7.992085 | 5.4 | -7.993348 | | | 5.2 | -8.030936 |
| | | | | | | 5.4 | -8.030274 |

TABLE IX. Potential-energy curves for the lowest singlet and triplet states of LiH in a magnetic field of 0.2 $B_0$ with R as the bond distance (in Bohr). Calculated at the CCSD(T) level with the uncontracted aug-cc-pVTZ basis set in a field perpendicular and parallel to the molecular bond axis.

| | | | B=0.2 $B_0$ | | | | |
|---|---|---|---|---|---|---|---|
| R | singlet$^{\perp}$ | R | $^1\Sigma^{\parallel}$ | R | triplet$^{\perp}$ | R | $^3\Pi^{\parallel}$ |
| 1.4 | -7.761330 | 1.4 | -7.729214 | 1.4 | -7.846115 | 1.4 | -7.859975 |
| 1.6 | -7.864046 | 1.6 | -7.837487 | 1.6 | -7.935177 | 1.6 | -7.951501 |
| 1.8 | -7.932842 | 1.8 | -7.910183 | 1.8 | -7.996147 | 1.8 | -8.013841 |
| 2.0 | -7.978007 | 2.0 | -7.958269 | 2.0 | -8.037908 | 2.0 | -8.056282 |
| 2.2 | -8.006685 | 2.2 | -7.989267 | 2.2 | -8.066383 | 2.2 | -8.084970 |
| 2.4 | -8.023861 | 2.6 | -8.019206 | 2.4 | -8.085625 | 2.4 | -8.104094 |
| 2.6 | -8.033009 | 2.8 | -8.024263 | 2.6 | -8.098439 | 2.6 | -8.116546 |
| 2.8 | -8.036557 | 2.9660 | -8.025356 | 2.8 | -8.106785 | 2.8 | -8.124351 |
| 2.8768 | -8.036811 | 3.0191 | -8.025249 | 3.0 | -8.112049 | 3.0 | -8.128937 |
| 3.0 | -8.036218 | 3.0248 | -8.025226 | 3.0191 | -8.112428 | 3.0191 | -8.129246 |
| 3.0191 | -8.036031 | 3.0 | -8.025310 | 3.0248 | -8.112539 | 3.0248 | -8.129335 |
| 3.0248 | -8.035970 | 3.2 | -8.023592 | 3.2 | -8.115211 | 3.2 | -8.131322 |
| 3.2 | -8.033210 | 3.4 | -8.019992 | 3.4 | -8.116965 | 3.4 | -8.132231 |
| 3.4 | -8.028400 | 3.6 | -8.015137 | 3.6 | -8.117800 | 3.4839 | -8.132303 |
| 3.6 | -8.022406 | 3.8 | -8.009476 | 3.8 | -8.118056 | 3.6 | -8.132183 |
| 3.8 | -8.015668 | 4.0 | -8.003331 | 4.0 | -8.117972 | 3.8 | -8.131546 |
| 4.0 | -8.008500 | 4.2 | -7.996933 | 4.2 | -8.117716 | 4.0 | -8.130577 |
| 4.2 | -8.001129 | 4.6 | -7.984004 | 4.6 | -8.117169 | 4.2 | -8.129456 |
| 4.6 | -7.986390 | 4.8 | -7.977680 | 4.8 | -8.117116 | 4.6 | -8.127184 |
| 4.8 | -7.979231 | 5.0 | -7.971541 | 5.0 | -8.117389 | 4.8 | -8.126151 |
| 5.0 | -7.972306 | 5.2 | -7.965631 | 5.2 | -8.117965 | 5.0 | -8.125225 |
| 5.2 | -7.965668 | 5.4 | -7.959984 | 5.4 | -8.118634 | 5.2 | -8.124412 |
| 5.4 | -7.959358 | | | | | 5.4 | -8.123710 |

TABLE X. Potential-energy curves for the lowest singlet and triplet states of LiH in a magnetic field of 0.4 $B_0$ with R as the bond distance (in Bohr). Calculated at the CCSD(T) level with the uncontracted aug-cc-pVTZ basis set in a field perpendicular and parallel to the molecular bond axis.

| | | | B=0.4 $B_0$ | | | | |
|---|---|---|---|---|---|---|---|
| R | singlet$^\perp$ | R | $^1\Sigma^\parallel$ | R | triplet$^\perp$ | R | $^3\Pi^\parallel$ |
| 1.4 | -7.749901 | 1.4 | -7.649242 | 1.4 | -7.971941 | 1.4 | -8.025563 |
| 1.6 | -7.843241 | 1.6 | -7.758299 | 1.6 | -8.057258 | 1.6 | -8.114904 |
| 1.8 | -7.903799 | 1.8 | -7.830700 | 1.8 | -8.115209 | 1.8 | -8.174916 |
| 2.0 | -7.941577 | 2.0 | -7.877863 | 2.0 | -8.155165 | 2.0 | -8.215017 |
| 2.2 | -7.963514 | 2.2 | -7.907583 | 2.2 | -8.183656 | 2.2 | -8.241438 |
| 2.4 | -7.974464 | 2.4 | -7.925231 | 2.4 | -8.204840 | 2.4 | -8.258428 |
| 2.6 | -7.977817 | 2.6 | -7.934516 | 2.6 | -8.220951 | 2.6 | -8.268919 |
| 2.6180 | -7.977834 | 2.8 | -7.938010 | 2.8 | -8.233267 | 2.8 | -8.274956 |
| 2.8 | -7.975957 | 2.8682 | -7.938216 | 3.0 | -8.242690 | 3.0 | -8.277981 |
| 3.0 | -7.970578 | 3.0191 | -7.937308 | 3.0191 | -8.243464 | 3.0191 | -8.278152 |
| 3.0191 | -7.969928 | 3.0248 | -7.937241 | 3.0248 | -8.243693 | 3.0248 | -8.278200 |
| 3.0248 | -7.969729 | 3.0 | -7.937514 | 3.2 | -8.249888 | 3.2 | -8.279016 |
| 3.2 | -7.962895 | 3.2 | -7.934293 | 3.4 | -8.255346 | 3.2536 | -8.279055 |
| 3.4 | -7.953779 | 3.4 | -7.929241 | 3.6 | -8.259418 | 3.4 | -8.278792 |
| 3.6 | -7.943855 | 3.6 | -7.922989 | 3.8 | -8.262375 | 3.6 | -8.277823 |
| 3.8 | -7.933582 | 3.8 | -7.915986 | 4.0 | -8.264431 | 3.8 | -8.276468 |
| 4.0 | -7.923305 | 4.0 | -7.908551 | 4.2 | -8.265771 | 4.0 | -8.274965 |
| 4.2 | -7.913300 | 4.2 | -7.900911 | 4.6 | -8.266921 | 4.2 | -8.273466 |
| 4.6 | -7.895058 | 4.6 | -7.885622 | 4.7606 | -8.266997 | 4.6 | -8.270801 |
| 4.8 | -7.887306 | 4.8 | -7.878169 | 4.8 | -8.266992 | 4.8 | -8.269700 |
| 5.0 | -7.880827 | 5.0 | -7.870926 | 5.0 | -8.266867 | 5.0 | -8.268759 |
| 5.2 | -7.875883 | 5.2 | -7.863929 | 5.2 | -8.266625 | 5.2 | -8.267967 |
| 5.4 | -7.872623 | 5.4 | -7.857201 | 5.4 | -8.266327 | 5.4 | -8.267309 |

TABLE XI. Potential-energy curves for the lowest triplet states of LiH at zero field and in a parallel magnetic field of 0.1 and 0.2 $B_0$ with R as the bond distance (in Bohr). Calculated at the CCSD(T) level with the uncontracted aug-cc-pVTZ basis set in a field perpendicular and parallel to the molecular bond axis.

| B=0.0 $B_0$ | | | | B=0.1 $B_0$ | | | | B=0.2 $B_0$ | | | |
|---|---|---|---|---|---|---|---|---|---|---|---|
| R | $^3\Pi^{\parallel}$ | R | $^3\Sigma^{\parallel}$ | R | $^3\Pi^{\parallel}$ | R | $^3\Sigma^{\parallel}$ | R | $^3\Pi^{\parallel}$ | R | $^3\Sigma^{\parallel}$ |
| 1.4 | -7.624431 | 1.4 | -7.661501 | 1.4 | -7.755434 | 1.6 | -7.836789 | 1.4 | -7.859975 | 1.4 | -7.809483 |
| 1.6 | -7.717706 | 1.6 | -7.752312 | 1.6 | -7.848053 | 1.8 | -7.898854 | 1.6 | -7.951501 | 1.6 | -7.898852 |
| 1.8 | -7.781722 | 1.8 | -7.814812 | 1.8 | -7.911464 | 2.0 | -7.941831 | 1.8 | -8.013841 | 1.8 | -7.960218 |
| 2.0 | -7.825766 | 2.0 | -7.858119 | 2.0 | -7.954943 | 2.2 | -7.971709 | 2.0 | -8.056282 | 2.0 | -8.002637 |
| 2.2 | -7.855986 | 2.2 | -7.888245 | 2.2 | -7.984627 | 2.4 | -7.992546 | 2.2 | -8.084970 | 2.2 | -8.032063 |
| 2.4 | -7.876563 | 2.4 | -7.909264 | 2.4 | -8.004695 | 2.6 | -8.007119 | 2.4 | -8.104094 | 2.4 | -8.052525 |
| 2.6 | -7.890381 | 2.6 | -7.923969 | 2.6 | -8.018032 | 2.8 | -8.017355 | 2.6 | -8.116546 | 2.6 | -8.066785 |
| 2.8 | -7.899452 | 2.8 | -7.934297 | 2.8 | -8.026652 | 3.0 | -8.024597 | 2.8 | -8.124351 | 2.8 | -8.076752 |
| 3.0 | -7.905198 | 3.0 | -7.941600 | 3.0 | -8.031978 | 3.2 | -8.029788 | 3.0 | -8.128937 | 3.0 | -8.083762 |
| 3.2 | -7.908630 | 3.0191 | -7.942176 | 3.0191 | -8.032354 | 3.4 | -8.033584 | 3.0191 | -8.129246 | 3.2 | -8.088750 |
| 3.4 | -7.910470 | 3.0248 | -7.942346 | 3.0248 | -8.032463 | 3.6 | -8.036443 | 3.0248 | -8.129335 | 3.4 | -8.092371 |
| 3.6 | -7.911237 | 3.2 | -7.946827 | 3.2 | -8.035025 | 3.8 | -8.038675 | 3.2 | -8.131322 | 3.6 | -8.095080 |
| 3.65 | -7.911306 | 3.4 | -7.950640 | 3.4 | -8.036517 | 4.0 | -8.040493 | 3.4 | -8.132231 | 3.8 | -8.097188 |
| 3.7 | -7.911337 | 3.6 | -7.953500 | 3.6 | -8.036971 | 4.2 | -8.042033 | 3.4839 | -8.132303 | 4.0 | -8.098907 |
| 3.7185 | -7.911339 | 3.8 | -7.955720 | 3.6237 | -8.036975 | 4.4 | -8.043383 | 3.6 | -8.132183 | 4.2 | -8.100375 |
| 3.75 | -7.911332 | 4.0 | -7.957515 | 3.8 | -8.036759 | 4.6 | -8.044595 | 3.8 | -8.131546 | 4.6 | -8.102858 |
| 3.8 | -7.911297 | 4.2 | -7.959025 | 4.0 | -8.036142 | 4.8 | -8.045696 | 4.0 | -8.130577 | 4.8 | -8.103948 |
| 3.85 | -7.911235 | 4.6 | -7.961509 | 4.2 | -8.035304 | 5.0 | -8.046703 | 4.2 | -8.129456 | 5.0 | -8.104958 |
| 3.9 | -7.911149 | 4.8 | -7.962567 | 4.4 | -8.034372 | 5.2 | -8.047621 | 4.6 | -8.127184 | 5.2 | -8.105889 |
| 3.95 | -7.911042 | 5.0 | -7.963531 | 4.6 | -8.033427 | 5.4 | -8.048454 | 4.8 | -8.126151 | 5.4 | -8.106742 |
| 4.0 | -7.910916 | 5.2 | -7.964407 | 4.8 | -8.032522 | | | 5.0 | -8.125225 | | |
| 4.2 | -7.910278 | 5.4 | -7.965201 | 5.0 | -8.031687 | | | 5.2 | -8.124412 | | |
| 4.6 | -7.908701 | | | 5.2 | -8.030936 | | | 5.4 | -8.123710 | | |
| 4.8 | -7.907903 | | | 5.4 | -8.030274 | | | | | | |
| 5.0 | -7.907151 | | | | | | | | | | |
| 5.2 | -7.906465 | | | | | | | | | | |
| 5.4 | -7.905850 | | | | | | | | | | |

TABLE XII. Equilibrium bond distances of the lowest singlet and triplet states of LiH as a function of the magnetic field (in Bohr). Calculated at the CCSD(T) level with the uncontracted aug-cc-pVTZ basis.

| $B/B_0$ | singlet$^\perp$ | $^1\Sigma^\parallel$ | triplet$^\perp$ | $^3\Pi^\parallel$ |
|---|---|---|---|---|
| 0 | 3.0249 | 3.0248 | | 3.7185 |
| 0.02 | 3.0244 | | | |
| 0.04 | 3.0187 | | | |
| 0.06 | 3.0094 | | | |
| 0.08 | 2.9969 | | | |
| 0.1 | 2.9801 | 3.0035 | | 3.6237 |
| 0.2 | 2.8768 | 2.9660 | | 3.4839 |
| 0.3 | 2.7474 | 2.9153 | | |
| 0.4 | 2.618 | 2.8682 | 4.7606 | 3.2536 |
| 0.5 | 2.4895 | 2.8229 | | |
| 0.6 | 2.3755 | 2.7795 | 3.8777 | 3.0945 |
| 0.8 | 2.1726 | 2.6978 | 3.3766 | 2.9856 |
| 1.0 | 2.0101 | 2.6292 | 3.0372 | 2.8649 |
| 1.2 | 1.8774 | 2.5677 | 2.7958 | 2.7114 |
| 1.4 | 1.7716 | 2.5045 | 2.6054 | 2.5664 |
| 1.6 | 1.6793 | 2.4496 | 2.4421 | 2.4453 |

TABLE XIII. HF-SCF, CCSD, CCSD(T), and total correlation energies (in Hartree) for the lowest singlet states of LiH in perpendicular and parallel orientation to the magnetic field. Calculated at the equilibrium geometries (in Bohr) of the respective field strength using the uncontraced aug-cc-pCVQZ basis set.

| | | | singlet$^{\perp}$ | | |
|---|---|---|---|---|---|
| B/$B_0$ | R | HF-SCF | CCSD | CCSD(T) | correlation |
| 0 | 3.0248 | -7.987280 | -8.068700 | -8.068853 | -0.081573 |
| 0.02 | 3.0244 | -7.986998 | -8.068413 | -8.068566 | -0.081568 |
| 0.04 | 3.0187 | -7.986156 | -8.067562 | -8.067716 | -0.081559 |
| 0.06 | 3.0094 | -7.984777 | -8.066174 | -8.066328 | -0.081550 |
| 0.08 | 2.9969 | -7.982891 | -8.064285 | -8.064438 | -0.081548 |
| 0.1 | 2.9801 | -7.980530 | -8.061935 | -8.062089 | -0.081560 |
| 0.2 | 2.8768 | -7.962696 | -8.044436 | -8.044606 | -0.081910 |
| 0.3 | 2.7474 | -7.936362 | -8.018914 | -8.019117 | -0.082755 |
| 0.4 | 2.6180 | -7.902554 | -7.986167 | -7.986411 | -0.083857 |
| 0.5 | 2.4895 | -7.862081 | -7.946844 | -7.947132 | -0.085051 |
| 0.6 | 2.3755 | -7.815765 | -7.901662 | -7.901990 | -0.086225 |
| 0.8 | 2.1726 | -7.708247 | -7.796277 | -7.796677 | -0.088430 |
| 1.0 | 2.0101 | -7.584292 | -7.674196 | -7.674652 | -0.090359 |
| 1.2 | 1.8774 | -7.446743 | -7.538272 | -7.538770 | -0.092027 |
| 1.4 | 1.7716 | -7.297530 | -7.390464 | -7.390994 | -0.093464 |
| 1.6 | 1.6793 | -7.137828 | -7.232003 | -7.232558 | -0.094700 |
| | | | singlet$^{\parallel}$ | | |
| B/$B_0$ | R | HF-SCF | CCSD | CCSD(T) | correlation |
| 0 | 3.0248 | -7.987280 | -8.068700 | -8.068853 | -0.081573 |
| 0.1 | 3.0035 | -7.977779 | -8.059080 | -8.059231 | -0.081453 |
| 0.2 | 2.9660 | -7.951644 | -8.032786 | -8.032934 | -0.081290 |
| 0.3 | 2.9153 | -7.912916 | -7.994055 | -7.994200 | -0.081284 |
| 0.4 | 2.8682 | -7.864731 | -7.946007 | -7.946151 | -0.081420 |
| 0.5 | 2.8229 | -7.809177 | -7.890691 | -7.890834 | -0.081657 |
| 0.6 | 2.7795 | -7.747647 | -7.829459 | -7.829602 | -0.081955 |
| 0.8 | 2.6978 | -7.610195 | -7.692693 | -7.692838 | -0.082643 |
| 1.0 | 2.6292 | -7.457243 | -7.540461 | -7.540609 | -0.083366 |
| 1.2 | 2.5677 | -7.291599 | -7.375537 | -7.375689 | -0.084090 |
| 1.4 | 2.5045 | -7.115137 | -7.199785 | -7.199942 | -0.084805 |
| 1.6 | 2.4496 | -6.929218 | -7.014550 | -7.014711 | -0.085493 |

TABLE XIV. HF-SCF, CCSD, CCSD(T), and total correlation energies (in Hartree) for the lowest singlet states of LiH in perpendicular and parallel orientation to the magnetic field. Calculated at a fixed distance of 3.0248 Bohr using the uncontraced aug-cc-pCVQZ basis set.

| | | singlet$^{\perp}$ | | |
|---|---|---|---|---|
| B/$B_0$ | HF-SCF | CCSD | CCSD(T) | correlation |
| 0 | -7.987280 | -8.068700 | -8.068853 | -0.081573 |
| 0.005 | -7.987262 | -8.068682 | -8.068835 | -0.081573 |
| 0.01 | -7.987209 | -8.068628 | -8.068781 | -0.081572 |
| 0.02 | -7.986998 | -8.068412 | -8.068565 | -0.081568 |
| 0.03 | -7.986647 | -8.068055 | -8.068208 | -0.081561 |
| 0.04 | -7.986158 | -8.067558 | -8.067711 | -0.081552 |
| 0.06 | -7.984778 | -8.066157 | -8.066310 | -0.081532 |
| 0.08 | -7.982881 | -8.064242 | -8.064394 | -0.081514 |
| 0.1 | -7.980494 | -8.061844 | -8.061997 | -0.081504 |
| 0.15 | -7.972544 | -8.053938 | -8.054095 | -0.081550 |
| 0.2 | -7.961965 | -8.043533 | -8.043697 | -0.081732 |
| 0.25 | -7.948858 | -8.030732 | -8.030909 | -0.082051 |
| 0.325 | -7.924488 | -8.007020 | -8.007222 | -0.082734 |
| 0.3 | -7.933238 | -8.015529 | -8.015721 | -0.082484 |
| 0.35 | -7.915118 | -7.997908 | -7.998120 | -0.083002 |
| 0.4 | -7.894546 | -7.977898 | -7.978129 | -0.083584 |
| 0.45 | -7.871607 | -7.955568 | -7.955822 | -0.084216 |
| 0.6 | -7.789704 | -7.875795 | -7.876129 | -0.086425 |
| 0.8 | -7.654741 | -7.744755 | -7.745266 | -0.090525 |
| 1.0 | -7.497385 | -7.593807 | -7.594726 | -0.097341 |
| 1.2 | -7.323415 | -7.430781 | -7.432776 | -0.109360 |
| 1.4 | -7.136736 | -7.260921 | -7.265375 | -0.128639 |
| 1.6 | -6.939927 | -7.084968 | -7.093093 | -0.153167 |
| | | singlet$^{\parallel}$ | | |
| B/$B_0$ | HF-SCF | CCSD | CCSD(T) | correlation |
| 0 | -7.987069 | -8.061331 | -8.061451 | -0.074382 |
| 0.1 | -7.977561 | -8.051647 | -8.051765 | -0.074204 |
| 0.2 | -7.951310 | -8.025114 | -8.025226 | -0.073917 |
| 0.3 | -7.912266 | -7.985909 | -7.986015 | -0.073749 |
| 0.4 | -7.863516 | -7.937140 | -7.937241 | -0.073725 |
| 0.5 | -7.807152 | -7.880861 | -7.880958 | -0.073806 |
| 0.6 | -7.744593 | -7.818455 | -7.818548 | -0.073955 |
| 0.8 | -7.604559 | -7.678823 | -7.678912 | -0.074353 |
| 1.0 | -7.448450 | -7.523161 | -7.523247 | -0.074797 |
| 1.2 | -7.279003 | -7.354148 | -7.354232 | -0.075229 |
| 1.4 | -7.097776 | -7.173320 | -7.173402 | -0.075626 |
| 1.6 | -6.905794 | -6.981692 | -6.981773 | -0.075979 |

TABLE XV. HF-SCF, CCSD, CCSD(T), and total correlation energies (in Hartree) for the lowest triplet states of LiH in perpendicular and parallel orientation to the magnetic field. Calculated at the equilibrium geometries (in Bohr) of the respective field strength using the uncontraced aug-cc-pCVQZ basis set.

| | | | triplet$^{\perp}$ | | |
|---|---|---|---|---|---|
| B/$B_0$ | R | HF-SCF | CCSD | CCSD(T) | correlation |
| 0.4 | 4.7606 | -8.226899 | -8.275302 | -8.275383 | -0.048484 |
| 0.6 | 3.8777 | -8.338929 | -8.389524 | -8.389631 | -0.050702 |
| 0.8 | 3.3766 | -8.428640 | -8.480979 | -8.481107 | -0.052466 |
| 1.0 | 3.0372 | -8.501194 | -8.554961 | -8.555105 | -0.053911 |
| 1.2 | 2.7958 | -8.559584 | -8.614519 | -8.614676 | -0.055092 |
| 1.4 | 2.6054 | -8.605230 | -8.661178 | -8.661344 | -0.056114 |
| 1.6 | 2.4421 | -8.639249 | -8.696124 | -8.696297 | -0.057048 |
| | | | triplet$^{\parallel}$ | | |
| B/$B_0$ | R | HF-SCF | CCSD | CCSD(T) | correlation |
| 0.4 | 4.7606 | -8.226899 | -8.275302 | -8.275383 | -0.048484 |
| 0.6 | 3.8777 | -8.338929 | -8.389524 | -8.389631 | -0.050702 |
| 0.8 | 3.3766 | -8.428640 | -8.480979 | -8.481107 | -0.052466 |
| 1.0 | 3.0372 | -8.501194 | -8.554961 | -8.555105 | -0.053911 |
| 1.2 | 2.7958 | -8.559584 | -8.614519 | -8.614676 | -0.055092 |
| 1.4 | 2.6054 | -8.605230 | -8.661178 | -8.661344 | -0.056114 |
| 1.6 | 2.4421 | -8.639249 | -8.696124 | -8.696297 | -0.057048 |

TABLE XVI. HF-SCF, CCSD, CCSD(T), and total correlation energies (in Hartree) for the lowest triplet states of LiH in perpendicular and parallel orientation to the magnetic field. Calculated at a fixed distance of 3.0248 Bohr using the uncontraced aug-cc-pCVQZ basis set.

| | | triplet$^{\perp}$ | | |
|---|---|---|---|---|
| B/$B_0$ | HF-SCF | CCSD | CCSD(T) | correlation |
| 0 | -7.903383 | -7.949165 | -7.949216 | -0.045832 |
| 0.005 | -7.908382 | -7.954170 | -7.954221 | -0.045839 |
| 0.01 | -7.913377 | -7.959184 | -7.959236 | -0.045858 |
| 0.02 | -7.923349 | -7.969228 | -7.969280 | -0.045931 |
| 0.03 | -7.933270 | -7.979256 | -7.979309 | -0.046039 |
| 0.04 | -7.943103 | -7.989217 | -7.989271 | -0.046168 |
| 0.06 | -7.962340 | -8.008729 | -8.008786 | -0.046446 |
| 0.08 | -7.980800 | -8.027447 | -8.027506 | -0.046706 |
| 0.1 | -7.998338 | -8.045208 | -8.045269 | -0.046931 |
| 0.15 | -8.037997 | -8.085259 | -8.085325 | -0.047328 |
| 0.2 | -8.072290 | -8.119695 | -8.119765 | -0.047475 |
| 0.25 | -8.102891 | -8.150112 | -8.150184 | -0.047293 |
| 0.3 | -8.133343 | -8.180659 | -8.180736 | -0.047393 |
| 0.325 | -8.149834 | -8.197821 | -8.197904 | -0.048070 |
| 0.35 | -8.167096 | -8.215852 | -8.215941 | -0.048845 |
| 0.4 | -8.202147 | -8.252045 | -8.252142 | -0.049995 |
| 0.45 | -8.236207 | -8.286852 | -8.286955 | -0.050748 |
| 0.6 | -8.327810 | -8.379821 | -8.379939 | -0.052130 |
| 0.8 | -8.425768 | -8.478868 | -8.479002 | -0.053234 |
| 1.0 | -8.501164 | -8.554962 | -8.555107 | -0.053943 |
| 1.2 | -8.558883 | -8.613162 | -8.613314 | -0.054431 |
| 1.4 | -8.601959 | -8.656601 | -8.656758 | -0.054798 |
| 1.6 | -8.632139 | -8.687074 | -8.687233 | -0.055094 |
| | | triplet$^{\parallel}$ | | |
| B/$B_0$ | HF-SCF | CCSD | CCSD(T) | correlation |
| 0 | -7.864566 | | -7.912781 | -0.048216 |
| 0.02 | -7.893358 | -7.941657 | -7.941717 | -0.048360 |
| 0.03 | -7.907000 | -7.955353 | -7.955414 | -0.048414 |
| 0.04 | -7.920148 | -7.968571 | -7.968632 | -0.048485 |
| 0.06 | -7.945110 | -7.993706 | -7.993769 | -0.048659 |
| 0.08 | -7.968535 | -8.017326 | -8.017392 | -0.048857 |
| 0.1 | -7.990661 | -8.039656 | -8.039725 | -0.049064 |
| 0.15 | -8.041408 | -8.090906 | -8.090982 | -0.049574 |
| 0.2 | -8.087002 | -8.136967 | -8.137050 | -0.050048 |
| 0.25 | -8.128546 | -8.178936 | -8.179026 | -0.050480 |
| 0.3 | -8.166760 | -8.217537 | -8.217634 | -0.050874 |
| 0.325 | -8.184785 | -8.235743 | -8.235843 | -0.051058 |
| 0.35 | -8.202158 | -8.253289 | -8.253392 | -0.051234 |
| 0.4 | -8.235120 | -8.286576 | -8.286685 | -0.051564 |
| 0.45 | -8.265936 | -8.317690 | -8.317804 | -0.051868 |
| 0.6 | -8.347578 | -8.400103 | -8.400232 | -0.052654 |
| 0.8 | -8.436503 | -8.489825 | -8.489969 | -0.053466 |
| 1.0 | -8.507834 | -8.561746 | -8.561898 | -0.054064 |
| 1.2 | -8.564589 | -8.618941 | -8.619099 | -0.054510 |
| 1.4 | -8.608365 | -8.663062 | -8.663222 | -0.054857 |
| 1.6 | -8.640260 | -8.695241 | -8.695402 | -0.055143 |

TABLE XVII. Correlation energy (in Hartree) for the triplet states in perpendicular and parallel orientation as a function of the bond distance R (in Bohr) at a field strength of 1.2 $B_0$. Calculated at the CCSD(T) level with the uncontracted aug-cc-pVTZ basis set.

| triplet$^{\perp}$ | | triplet$^{\parallel}$ | |
|---|---|---|---|
| R | correlation | R | correlation |
| 1.4 | -0.050365 | 1.4 | -0.051825 |
| 1.5 | -0.049769 | 1.6 | -0.049912 |
| 1.6 | -0.049202 | 1.8 | -0.048389 |
| 1.8 | -0.048175 | 2.0 | -0.047195 |
| 2.0 | -0.047278 | 2.2 | -0.046234 |
| 2.2 | -0.046484 | 2.4 | -0.045423 |
| 2.4 | -0.045760 | 2.6 | -0.044711 |
| 2.6 | -0.045075 | 2.7114 | -0.044347 |
| 2.7958 | -0.044423 | 2.8 | -0.044072 |
| 2.8 | -0.044409 | 3.0 | -0.043494 |
| 3.0 | -0.043768 | 3.0191 | -0.043442 |
| 3.0191 | -0.043709 | 3.0248 | -0.043426 |
| 3.0248 | -0.043692 | 3.2 | -0.042975 |
| 3.2 | -0.043173 | 3.4 | -0.042515 |
| 3.4 | -0.042642 | 3.6 | -0.042114 |
| 3.6 | -0.042182 | 3.8 | -0.041773 |
| 3.8 | -0.041794 | 4.0 | -0.041488 |
| 4.0 | -0.041474 | 4.2 | -0.041255 |
| 4.2 | -0.041217 | 4.6 | -0.040921 |
| 4.6 | -0.040863 | 4.8 | -0.040805 |
| 4.8 | -0.040748 | 5.0 | -0.040714 |
| 5.0 | -0.040662 | 5.2 | -0.040643 |
| 5.2 | -0.040597 | 5.4 | -0.040588 |
| 5.4 | -0.040549 | | |

TABLE XVIII. Basis-set convergence for the correlation energy (in Hartree) of the lithium $^2$P state in CCSD(T) calculations with finite magnetic fields. All basis sets were uncontracted

| B/$B_0$ | aug-cc-pVTZ | B/$B_0$ | aug-cc-pVQZ | aug-cc-pV5Z | cc-pVTZ |
|---|---|---|---|---|---|
| 0.005 | -0.037309 | 0.02 | -0.039749 | -0.040785 | -0.037313 |
| 0.01 | -0.037312 | 0.05 | -0.039863 | -0.040911 | -0.037410 |
| 0.02 | -0.037328 | 0.07 | -0.039971 | -0.041032 | -0.037503 |
| 0.04 | -0.037384 | 0.1 | -0.040159 | -0.041242 | -0.037661 |
| 0.06 | -0.037466 | 0.2 | -0.040858 | -0.042044 | -0.038234 |
| 0.08 | -0.037562 | 0.3 | -0.041570 | -0.042876 | -0.038802 |
| 0.1 | -0.037667 | 0.4 | -0.042240 | -0.043673 | -0.039267 |
| 0.12 | -0.037775 | 0.5 | -0.042842 | -0.044417 | -0.039619 |
| 0.14 | -0.037886 | 0.6 | -0.043374 | -0.045103 | -0.039880 |
| 0.16 | -0.037997 | 0.8 | -0.044231 | -0.046301 | -0.040196 |
| 0.18 | -0.038108 | 1 | -0.044811 | -0.047280 | -0.040316 |
| 0.2 | -0.038218 | 1.2 | -0.045143 | -0.048054 | -0.040292 |
| 0.3 | -0.038742 | 1.4 | -0.045279 | -0.048648 | -0.040144 |
| 0.4 | -0.039195 | 1.6 | -0.045268 | -0.049093 | -0.039892 |
| 0.5 | -0.039567 | | | | |
| 0.6 | -0.039854 | | | | |
| 0.7 | -0.040063 | | | | |
| 0.8 | -0.040203 | | | | |
| 0.9 | -0.040287 | | | | |
| 1.0 | -0.040326 | | | | |
| 1.1 | -0.040328 | | | | |
| 1.2 | -0.040297 | | | | |
| 1.3 | -0.040235 | | | | |
| 1.4 | -0.040147 | | | | |
| 1.5 | -0.040034 | | | | |
| 1.6 | -0.039901 | | | | |

| B/$B_0$ | cc-pVQZ | cc-pV5Z | aug-cc-pCVTZ | aug-cc-pCVQZ | cc-pCVTZ | cc-pCVQZ |
|---|---|---|---|---|---|---|
| 0.02 | -0.039619 | -0.040748 | -0.042223 | -0.043875 | -0.042206 | -0.043871 |
| 0.05 | -0.039734 | -0.040875 | -0.042325 | -0.044000 | -0.042310 | -0.043997 |
| 0.07 | -0.039844 | -0.040998 | -0.042422 | -0.044119 | -0.042410 | -0.044119 |
| 0.1 | -0.040036 | -0.041212 | -0.042590 | -0.044327 | -0.042581 | -0.044331 |
| 0.2 | -0.040763 | -0.042025 | -0.043203 | -0.045112 | -0.043209 | -0.045146 |
| 0.3 | -0.041476 | -0.042846 | -0.043806 | -0.045934 | -0.043851 | -0.045970 |
| 0.4 | -0.042124 | -0.043635 | -0.044355 | -0.046733 | -0.044403 | -0.046746 |
| 0.5 | -0.042709 | -0.044382 | -0.044834 | -0.047482 | -0.044851 | -0.047476 |
| 0.6 | -0.043234 | -0.045074 | -0.045241 | -0.048177 | -0.045217 | -0.048162 |
| 0.8 | -0.044088 | -0.046271 | -0.045852 | -0.049408 | -0.045776 | -0.049388 |
| 1 | -0.044662 | -0.047224 | -0.046277 | -0.050420 | -0.046189 | -0.050390 |
| 1.2 | -0.044984 | -0.047964 | -0.046598 | -0.051239 | -0.046518 | -0.051197 |
| 1.4 | -0.045113 | -0.048526 | -0.046852 | -0.051917 | -0.046782 | -0.051866 |
| 1.6 | -0.045096 | -0.048942 | -0.047053 | -0.052499 | -0.046990 | -0.052444 |

TABLE XIX. Basis-set convergence for the correlation energy (in Hartree) of the beryllium $^1$D state in CCSD(T) calculations with finite magnetic fields. All basis sets were uncontracted

| $B/B_0$ | cc-pVTZ | cc-pCVTZ | aug-pVTZ | aug-cc-pCVTZ |
|---|---|---|---|---|
| 0 | -0.078174 | -0.082784 | -0.092590 | -0.097135 |
| 0.00005 | -0.078175 | -0.082784 | | -0.097135 |
| 0.05 | -0.078607 | -0.083220 | | -0.096906 |
| 0.1 | -0.079794 | -0.084417 | -0.091584 | -0.096149 |
| 0.2 | -0.083139 | -0.087795 | -0.089254 | -0.093871 |
| 0.3 | -0.085688 | -0.090397 | | -0.092282 |
| 0.4 | -0.086755 | -0.091535 | -0.086714 | -0.091469 |
| 0.6 | -0.086278 | -0.091232 | -0.085303 | -0.090224 |
| 0.8 | -0.084334 | -0.089487 | -0.083638 | -0.088756 |
| 1.0 | -0.081595 | -0.086971 | -0.081463 | -0.086803 |
| 1.2 | -0.078265 | -0.083885 | -0.078620 | -0.084204 |
| 1.4 | -0.074624 | -0.080504 | -0.075280 | -0.081128 |
| $B/B_0$ | cc-pVQZ | cc-pCVQZ | aug-pVQZ | aug-cc-pCVQZ |
| 0 | -0.083421 | -0.087718 | -0.096936 | -0.101144 |
| 0.00005 | -0.083422 | -0.087718 | -0.096936 | -0.101144 |
| 0.05 | -0.083908 | -0.088207 | -0.096399 | -0.100612 |
| 0.1 | -0.085188 | -0.089498 | -0.095096 | -0.099323 |
| 0.2 | -0.088417 | -0.092762 | -0.092761 | -0.097034 |
| 0.3 | -0.090639 | -0.095032 | -0.091849 | -0.096182 |
| 0.4 | -0.091629 | -0.096083 | -0.091575 | -0.095976 |
| 0.6 | -0.091744 | -0.096353 | -0.091526 | -0.096086 |
| 0.8 | -0.091363 | -0.096159 | -0.091496 | -0.096239 |
| 1.0 | -0.091122 | -0.096130 | -0.091363 | -0.096313 |
| 1.2 | -0.090952 | -0.096199 | -0.091188 | -0.096368 |
| 1.4 | -0.090750 | -0.096261 | -0.090973 | -0.096406 |
| $B/B_0$ | cc-pV5Z | cc-pCV5Z | aug-pV5Z | |
| 0 | -0.089042 | -0.092995 | -0.099821 | |
| 0.00005 | -0.089042 | -0.092995 | -0.099822 | |
| 0.05 | -0.089477 | -0.093422 | -0.098660 | |
| 0.1 | -0.090502 | -0.094429 | -0.096617 | |
| 0.2 | -0.092472 | -0.096326 | -0.094296 | |
| 0.3 | -0.093309 | -0.097096 | -0.093517 | |
| 0.4 | -0.093410 | -0.097192 | -0.093250 | |
| 0.6 | -0.093262 | -0.097171 | -0.093142 | |
| 0.8 | -0.093300 | -0.097434 | -0.093226 | |
| 1 | -0.093439 | -0.097787 | -0.093380 | |
| 1.2 | -0.093568 | -0.098099 | -0.093548 | |
| 1.4 | -0.093635 | -0.098351 | -0.093707 | |

TABLE XX. Basis-set convergence for the correlation energy (in Hartree) of the $^2$S, $^2$P, $^2$D, and $^2$F states of sodium in CCSD(T) calculations with finite magnetic fields. All basis sets were uncontracted.

| | | aug-pCVTZ | | |
|---|---|---|---|---|
| B/$B_0$ | $^2$S | $^2$P | $^2$D | $^2$F |
| 0 | -0.336936 | -0.333371 | | |
| 0.1 | -0.337417 | -0.333994 | -0.332617 | |
| 0.2 | -0.338137 | -0.334811 | -0.333389 | -0.332055 |
| 0.3 | -0.338639 | -0.335457 | -0.334152 | -0.332040 |
| 0.4 | -0.338894 | -0.335956 | -0.334695 | -0.332095 |
| 0.5 | -0.338952 | -0.336299 | -0.334735 | -0.331926 |
| 0.6 | -0.338835 | -0.336468 | -0.334453 | -0.331514 |
| 0.7 | | | -0.334019 | -0.330972 |
| 0.8 | -0.338128 | -0.336403 | -0.333530 | -0.330348 |
| 0.9 | | | -0.333049 | -0.329674 |
| 1.0 | -0.337055 | -0.336152 | -0.332639 | |
| 1.1 | | | -0.332387 | |
| 1.2 | -0.335887 | -0.335977 | | |
| 1.4 | -0.334782 | -0.335946 | | |
| 1.6 | | -0.336029 | | |
| | | aug-pCVQZ | | |
| B/$B_0$ | $^2$S | $^2$P | $^2$D | $^2$F |
| 0 | -0.367533 | -0.363314 | | |
| 0.000000001 | | -0.363314 | -0.361901 | |
| 0.005 | -0.367535 | | | |
| 0.05 | | | | |
| 0.01 | -0.367540 | | | |
| 0.02 | -0.367565 | | | |
| 0.04 | -0.367656 | | | |
| 0.06 | -0.367792 | | | |
| 0.08 | -0.367958 | | | |
| 0.1 | -0.368142 | -0.364165 | -0.362357 | -0.361705 |
| 0.12 | -0.368334 | | | |
| 0.14 | -0.368527 | | | |
| 0.16 | -0.368717 | | | |
| 0.18 | -0.368900 | | | |
| 0.2 | -0.369072 | -0.365361 | -0.363480 | -0.361944 |
| 0.3 | -0.369722 | -0.366505 | -0.364640 | -0.362456 |
| 0.4 | -0.369965 | -0.367512 | -0.365782 | -0.362885 |
| 0.5 | -0.369847 | -0.368370 | -0.366854 | -0.363371 |
| 0.6 | -0.369492 | -0.369112 | -0.367740 | -0.363751 |
| 0.7 | -0.369014 | -0.369742 | -0.368394 | -0.363796 |
| 0.8 | -0.368473 | -0.370244 | -0.368843 | -0.363532 |
| 0.9 | -0.367894 | -0.370614 | | -0.363080 |
| 1.0 | -0.367285 | -0.370867 | -0.369340 | -0.362529 |
| 1.1 | -0.366653 | -0.371037 | | -0.361939 |
| 1.2 | -0.366005 | | -0.369638 | |
| 1.3 | -0.365351 | | -0.370050 | |
| 1.4 | -0.364700 | | -0.370743 | |

TABLE XXI. Basis-set convergence for the correlation energy (in Hartree) of the triplet state of LiH in perpendicular orientation at a fixed bond distance of R=3.0248 Bohr, calculated at the CCSD(T) level with finite magnetic fields. All basis sets were uncontracted.

| B | aug-cc-pVTZ | aug-cc-pCVQZ |
|---|---|---|
| 0 | -0.039178 | -0.045781 |
| 0.005 | -0.039184 | -0.045788 |
| 0.01 | -0.039202 | -0.045807 |
| 0.02 | -0.039271 | -0.045900 |
| 0.03 | -0.039372 | -0.046000 |
| 0.04 | -0.039494 | -0.046114 |
| 0.06 | -0.039752 | -0.046389 |
| 0.08 | -0.039992 | -0.046647 |
| 0.1 | -0.040225 | -0.046869 |
| 0.15 | -0.040534 | -0.047262 |
| 0.2 | -0.040616 | -0.047404 |
| 0.25 | -0.040339 | -0.047221 |
| 0.3 | -0.040219 | -0.047317 |
| 0.325 | -0.040787 | -0.047987 |
| 0.35 | -0.041482 | -0.048756 |
| 0.4 | -0.042481 | -0.049898 |
| 0.45 | -0.043074 | -0.050645 |
| 0.6 | -0.043929 | -0.052011 |
| 0.8 | -0.044215 | -0.053101 |
| 1.0 | -0.044060 | -0.053799 |
| 1.2 | -0.043692 | -0.054279 |
| 1.4 | -0.043165 | -0.054642 |
| 1.6 | -0.042482 | -0.054935 |

TABLE XXII. Binding energy (in kJ/mol) for the singlet state of LiH in perpendicular orientation as a function of the magnetic field. Calculations were performed using the uncontracted aug-cc-pCVQZ basis set.

| $B/B_0$ | CCSD(T) BSSE corrected | HF-SCF BSSE corrected | CCSD(T) not corrected | HF-SCF not corrected | CCSD(T) not correted dissociation Li→$^2$P | CCSD(T) not corrected dissociation Li →$^2$S |
|---|---|---|---|---|---|---|
| 0 | 241.675 | 143.345 | 241.692 | 143.347 | | 241.688 |
| 0.02 | | | 242.797 | 144.488 | 396.216 | 242.797 |
| 0.04 | | | 246.070 | 147.848 | 376.811 | 246.070 |
| 0.06 | | | 251.360 | 153.257 | 361.081 | 251.360 |
| 0.08 | | | 258.480 | 160.506 | 348.245 | 258.480 |
| 0.1 | | | 267.248 | 169.383 | 337.696 | 267.248 |
| 0.2 | 307.224 | 210.675 | 307.343 | 210.730 | 307.343 | 330.222 |
| 0.3 | 298.082 | 201.516 | 298.352 | 201.679 | 298.352 | 413.370 |
| 0.4 | 298.083 | 200.769 | 298.681 | 201.210 | 298.681 | 505.095 |
| 0.5 | 301.858 | 203.447 | 302.929 | 204.292 | 302.929 | 599.097 |
| 0.6 | 307.416 | 207.841 | 309.113 | 209.218 | 309.113 | 692.651 |
| 0.8 | 321.151 | 219.299 | 324.284 | 221.831 | 324.284 | 875.808 |
| 1.0 | 336.350 | 232.487 | 341.223 | 236.361 | 341.223 | 1053.391 |
| 1.2 | 352.611 | 246.991 | 360.412 | 253.321 | 360.412 | 1224.499 |
| 1.4 | 369.962 | 262.832 | 383.600 | 274.517 | 383.600 | 1388.762 |
| 1.6 | 387.966 | 279.503 | 411.368 | 300.491 | 411.368 | 1547.627 |

TABLE XXIII. Binding energy (in kJ/mol) for the singlet state of $He_3$ in perpendicular orientation as a function of the magnetic field. Calculations were performed using the uncontracted aug-cc-pCVQZ basis set.

| $B/B_0$ | CCSD(T) BSSE corrected | HF-SCF BSSE corrected | CCSD(T) not corrected | HF-SCF not corrected |
|---|---|---|---|---|
| 0 | 0.237 | -0.170 | 0.247 | -0.166 |
| 0.2 | 0.399 | -0.261 | 0.414 | -0.253 |
| 0.4 | 1.070 | -0.573 | 1.152 | -0.508 |
| 0.6 | 2.678 | -0.998 | 2.884 | -0.824 |
| 0.8 | 5.737 | -1.202 | 6.015 | -0.970 |
| 1.0 | 10.661 | -0.478 | 10.913 | -0.283 |
| 1.2 | 17.694 | 1.491 | 17.953 | 1.673 |
| 1.4 | 26.869 | 5.156 | 27.475 | 5.648 |
| 1.6 | 38.035 | 10.634 | 39.611 | 12.038 |
| 1.8 | 50.889 | 17.716 | 54.232 | 20.807 |
| 2.0 | 64.996 | 26.420 | 71.081 | 32.161 |

TABLE XXIV: Comparison of total energies ($E_{\rm tot}$), and correlation energies ($E_{\rm corr}$) for He, Li, Be, and $H_2$ with published data. All calculations were performed using the uncontracted aug-cc-pCVQZ basis set except for He where the uncontracted d-aug-cc-pVQZ basis set was employed.

| | this work | | Literature | | Differences | |
|---|---|---|---|---|---|---|
| He $^1S$, $[1_0{}^1(0)^+]$ | | | | | | |
| B/$B_0$ | $E_{\rm tot}$ | $E_{\rm corr}$ | $E_{\rm tot}$ (Ref. 1) | $E_{\rm corr}$ (Ref. 2) | $\Delta E_{\rm tot}$ | $\Delta E_{\rm corr}$ |
| 0.0 | -2.902836 | -0.041289 | -2.903351 | -0.041 | -5.1E-04 | 2.9E-04 |
| 0.4 | -2.871958 | -0.041083 | -2.872501 | | -5.4E-04 | |
| 0.5 | -2.855304 | -0.040998 | -2.855859 | | -5.6E-04 | |
| 0.8 | -2.787419 | -0.040756 | -2.787556 | -0.041 | -1.4E-04 | -2.4E-04 |
| 1.0 | -2.729313 | -0.040631 | -2.729508 | | -2.0E-04 | |
| 2.0 | -2.328190 | -0.040446 | -2.329780 | -0.041 | -1.6E-03 | -5.5E-04 |
| He $^3P$, $[1_{-1}{}^3(-1)^+]$ | | | | | | |
| B/$B_0$ | $E_{\rm tot}$ | $E_{\rm corr}$ | $E_{\rm tot}$ (Ref. 3) | $E_{\rm corr}$ (Ref. 2) | $\Delta E_{\rm tot}$ | $\Delta E_{\rm corr}$ |
| 0.0 | -2.130862 | -0.001889 | -2.133164 | -0.0017 | -2.3E-03 | 1.9E-04 |
| 0.4 | -2.537685 | -0.004090 | -2.540763 | | -3.1E-03 | |
| 0.5 | -2.617648 | -0.004506 | -2.620021 | | -2.4E-03 | |
| 0.8 | -2.833704 | -0.005374 | -2.835619 | -0.0054 | -1.9E-03 | -2.6E-05 |
| 1.0 | -2.961129 | -0.005757 | -2.965504 | | -4.4E-03 | |
| 2.0 | -3.488146 | -0.006618 | -3.508911 | -0.0068 | -2.1E-02 | -1.8E-04 |
| Li $^2S$, $[1_{-1/2}{}^2(0)^+]$ | | | | | | |
| B/$B_0$ | $E_{\rm tot}$ | $E_{\rm corr}$ | $E_{\rm tot}$ (Ref. 4) | | $\Delta E_{\rm tot}$ | |
| 0.0 | -7.476841 | -0.044116 | -7.477766 | | -9.2E-04 | |
| 0.02 | -7.486232 | -0.044124 | -7.490983 | | -4.8E-03 | |
| 0.1 | -7.512818 | -0.044285 | -7.517154 | | -4.3E-03 | |
| 0.2 | -7.528508 | -0.044591 | -7.533495 | | -5.0E-03 | |
| 0.5 | -7.521859 | -0.045316 | -7.528055 | | -6.2E-03 | |
| 1.0 | -7.442729 | -0.045769 | -7.458550 | | -1.6E-02 | |
| Li $^2P$, $[1_{-1/2}{}^2(-1)^+]$ | | | | | | |
| B/$B_0$ | $E_{\rm tot}$ | $E_{\rm corr}$ | $E_{\rm tot}$ (Ref. 4) | | $\Delta E_{\rm tot}$ | |
| 0.1 | -7.485985 | -0.044327 | -7.484773 | | 1.2E-03 | |
| 0.2 | -7.537222 | -0.045112 | -7.536032 | | 1.2E-03 | |
| 0.5 | -7.634663 | -0.047482 | -7.634547 | | 1.2E-04 | |
| 1.0 | -7.713979 | -0.050420 | -7.716679 | | -2.7E-03 | |
| 2.0 | -7.687095 | -0.053487 | -7.715709 | | -2.9E-02 | |
| Be $^1S$, $[1_0{}^1(0)^+]$ | | | | | | |
| B/$B_0$ | $E_{\rm tot}$ | $E_{\rm corr}$ | $E_{\rm tot}$ (Ref. 5) | | $\Delta E_{\rm tot}$ | |
| 0.0 | -14.665797 | -0.092810 | -14.66287 | | 2.9E-03 | |
| 0.1 | -14.652565 | -0.093634 | -14.64955 | | 3.0E-03 | |
| 0.2 | -14.615754 | -0.095675 | -14.61160 | | 4.2E-03 | |
| 0.4 | -14.492014 | -0.102062 | -14.48793 | | 4.1E-03 | |
| 0.6 | -14.327057 | -0.112154 | -14.32037 | | 6.7E-03 | |
| 0.7 | -14.235587 | -0.119248 | -14.22625 | | 9.3E-03 | |

TABLE XXIV: Comparison of total energies ($E_{\text{tot}}$), and correlation energies ($E_{\text{corr}}$) for He, Li, Be, and $H_2$ with published data (continued). All calculations were performed using the uncontracted aug-cc-pCVQZ basis set except for He where the uncontracted d-aug-cc-pVQZ basis set was employed.

| | | this work | | Literature | | Differences | |
|---|---|---|---|---|---|---|---|
| Be $^3P$, $[1_{-1}{}^3(-1)^+]$ | | | | | | | |
| $B/B_0$ | | $E_{\text{tot}}$ | $E_{\text{corr}}$ | $E_{\text{tot}}$ (Ref. 5) | | $\Delta E_{\text{tot}}$ | |
| 0.2 | | -14.804703 | -0.054143 | -14.80065 | | 4.1E-03 | |
| 0.4 | | -14.959725 | -0.055267 | -14.95507 | | 4.7E-03 | |
| 0.6 | | -15.067756 | -0.056669 | -15.06181 | | 5.9E-03 | |
| 0.8 | | -15.146937 | -0.058182 | -15.13834 | | 8.6E-03 | |
| 1.0 | | -15.206760 | -0.059713 | -15.19348 | | 1.3E-02 | |
| $H_2$ $^1\Sigma_g$, parallel | | | | | | | |
| $B/B_0$ | R | $E_{\text{tot}}$ | $E_{\text{corr}}$ | $E_{\text{tot}}$ (Ref. 6) | $E_{\text{corr}}$ (Ref. 2) | $\Delta E_{\text{tot}}$ | $\Delta E_{\text{corr}}$ |
| 0.0 | 1.40 | -1.173974 | -0.040471 | -1.173436 | -0.0397 | 5.4E-04 | 7.7E-04 |
| 0.01 | 1.40 | -1.173936 | -0.040472 | -1.173396 | -0.0397 | 5.4E-04 | 7.7E-04 |
| 0.1 | 1.39 | -1.170173 | -0.040483 | -1.169652 | -0.0398 | 5.2E-04 | 6.8E-04 |
| 0.2 | 1.39 | -1.159091 | -0.040691 | -1.158766 | -0.0402 | 3.3E-04 | 4.9E-04 |
| 0.5 | 1.33 | -1.089187 | -0.041435 | -1.089082 | -0.0411 | 1.0E-04 | 3.4E-04 |
| 1.0 | 1.24 | -0.890424 | -0.043246 | -0.890336 | -0.0429 | 8.8E-05 | 3.5E-04 |
| 2.0 | 1.09 | -0.334922 | -0.046451 | -0.335574 | -0.0465 | -6.5E-04 | -4.9E-05 |
| 5.0 | 0.86 | 1.809273 | -0.052836 | 1.801212 | -0.0541 | -8.1E-03 | -1.3E-03 |
| $H_2$ $^3\Sigma_u$, parallel | | | | | | | |
| $B/B_0$ | R | $E_{\text{tot}}$ | $E_{\text{corr}}$ | $E_{\text{tot}}$ (Ref. 6) | $E_{\text{corr}}$ (Ref. 2) | $\Delta E_{\text{tot}}$ | $\Delta E_{\text{corr}}$ |
| 0.0 | 7.9 | -0.999934 | -0.000034 | -1.000017 | -0.00003 | -8.3E-05 | 3.6E-06 |
| 0.01 | 7.9 | -1.009884 | -0.000034 | -1.009966 | -0.00006 | -8.2E-05 | -2.6E-05 |
| 0.1 | 7.8 | -1.094985 | -0.000035 | -1.095063 | -0.00003 | -7.8E-05 | 5.1E-06 |
| 0.2 | 7.7 | -1.180676 | -0.000035 | -1.180776 | -0.00003 | -1.0E-04 | 4.7E-06 |
| 0.5 | 7.4 | -1.394253 | -0.000031 | -1.394434 | -0.00003 | -1.8E-04 | 6.2E-07 |
| 1.0 | 7.5 | -1.661445 | -0.000015 | -1.662309 | -0.00002 | -8.6E-04 | -4.8E-06 |
| $H_2$ $^3\Pi_u$, parallel | | | | | | | |
| $B/B_0$ | R | $E_{\text{tot}}$ | $E_{\text{corr}}$ | $E_{\text{tot}}$ (Ref. 7) | $E_{\text{corr}}$ (Ref. 2) | $\Delta E_{\text{tot}}$ | $\Delta E_{\text{corr}}$ |
| 2.0 | 1.35 | -1.883691 | -0.010292 | -1.889260 | -0.0105 | -5.6E-03 | -2.1E-04 |
| 5.0 | 1.03 | -2.623070 | -0.012831 | -2.658910 | -0.0138 | -3.6E-02 | -9.7E-04 |

## REFERENCES

[1]W. Becken, P. Schmelcher, and F. K. Diakonos, "The helium atom in a strong magnetic field," J. Phys. B: At. Mol. Opt. Phys. **32**, 1557–1584 (1999).

[2]P. Schmelcher, M. V. Ivanov, and W. Becken, "Exchange and correlation energies of ground states of atoms and molecules in strong magnetic fields," Phys. Rev. A **59**, 3424 (1999).

[3]W. Becken and P. Schmelcher, "Non-zero angular momentum states of the helium atom in a strong magnetic field," J. Phys. B: At. Mol. Opt. Phys. **33**, 545–568 (2000).

[4]O.-A. Al-Hujaj and P. Schmelcher, "Lithium in strong magnetic fields," Phys. Rev. A **70**, 033411 (2004).

[5]X. X. Guan, B. W. Li, and K. T. Taylor, "Ionization energies of beryllium in strong magnetic fields: a frozen core approximation," J. Phys. B: At. Mol. Opt. Phys. **36**, 2465–2477 (2003).

[6]T. Detmer, P. Schmelcher, F. K. Diakonos, and L. S. Cederbaum, "Hydrogen molecule in magnetic fields: The ground states of the Sigma manifold of the parallel configuration," Phys. Rev. A **56**, 1825–1838 (1997).

[7]T. Detmer, P. Schmelcher, and L. S. Cederbaum, "Hydrogen molecule in a magnetic field: The lowest states of the Pi manifold and the global ground state of the parallel configuration," Phys. Rev. A **57**, 1767–1777 (1998).
